# Supplementary material for: Coding Schemes for Securing Cyber-Physical Systems Against Stealthy Data Injection Attacks
Source: arXiv:1605.08962 source file (2016-05-29)
Supplement: Supplementary file 1 [file appendix.tex]

\appendix
\section{Appendix}
\label{appendix}
%\begin{appendices}
\textit{Proof of Theorem~\ref{code}}

\begin{proof}
Assume the vector $y^{*}$ satisfies $y^{*} =Cv$ 
%(for different norm of vector $y^*$, $y^{*} =a Cv, a \in \mathbb{R}$, the following proof still holds), 
$v$ is a reachable state of the controllability matrix associated with (A-KCA, K), Collarary~\ref{stealth_fi} holds, so there exists a sequence of injections $y^{a}_0, ..., y^{a}_{n-1}$, such that: 
\begin{align}
\begin{split}
&\Delta e_{k+1} = (A-KCA) \Delta e_{k} - Ky^{a}_{k+1},
\Delta e_{n-1}=v,
\end{split}
\label{ya}
\end{align}
where $n$ is the dimension of state space. 
Define
\footnotesize
\begin{align*}
M=\max_{k=0,\dots,n-1}\|\Delta z_k\|, y^a_{n+i}=y^a_i -\lambda^{i+1}y^*,  i=0,1,\dots,
%\label{M}
\end{align*} 
\normalsize
it is shown by~\cite{false_injection} that $\|\Delta z_{n+i}\| =\|\Delta z_i\| \leq M, i=0,1,\dots$ for the system before sensor output transformation.
%%%%%%%%%%%%%%%%%%%%%%%%%%
%%%%%%%%%%%%%%%%%%%%%%%%%%

Considering an invertible matrix $\Sigma$, let 
\begin{align}
\Delta y=\Sigma Cv-y^*,  y*=a Cv, \forall a\in \mathbb{R}.
\label{delta_y}
\end{align}
With the condition~\eqref{Sigma_c}, $\Sigma Cv-Cv \neq 0$ implies $\Sigma Cv- aCv\neq 0$. 
Thus $\Delta y \neq 0$ holds if $\Sigma$ satisfies Theorem 2. 
%Even when the attacker designs the injection sequence based on $a \neq 1$, condition~\eqref{Sigma_c} guarantees that . 

When the attacker %does not know $\Sigma$ and 
injects the above stealth sequence $y^a_k, k=0,1,\dots$ to $Y_k$ of~\eqref{sig_y},
%$\mathbf{y}^a_0, \cdots, \mathbf{y}^a_{n-1}, \cdots, \mathbf{y}^a_{n+i}=\mathbf{y}^a_i-\lambda^{i+1}\mathbf{y}^*, i=0,1,\cdots$ for the original system, 
%the first $n-1$ steps of $\Delta e'_k$ is $\Delta e'_0=-K'y^a_0, \dots, \Delta e'_{n-1}$.
for the coded sensor output system, $\Delta e'_0=-K'y^a_0$, %with a similar argument as the original system, 
the dynamics of $\Delta e'_k, \Delta z'_k$ satisfy:
\footnotesize
\begin{align}
\begin{split}
&\Delta e'_{k+1} = \tilde{A} \Delta e'_{k} - K'y^{a}_{k+1},\Delta z'_{k+1}=\Sigma CA\Delta e'_k+ y^a_k,\\
& \Delta e'_{n-1}= v+\Delta v,\tilde{A}=A-K'\Sigma CA,
%&\Delta \mathbf{e}'_{n-1}=\mathbf{v}+\Delta \mathbf{v},
\end{split}
\label{ez}
\end{align}
\normalsize
where $n$ is the dimension of state space. 
Note that $n$ is a finite number, and the injection $y^a_k$ are finite in the first $n-1$ steps, thus both 
$\Delta e'_k, \Delta z'_k$ are finite in the first $n-1$ steps.  
%For simplicity of proof, assume that 
%\begin{align*}
%\Delta e'_{n-1}= v+\Delta v,\tilde{A}=A-K'\Sigma CA,
%\end{align*}

In the following proof, we will show that when $\Delta y \neq 0$, $\Delta z'_k$ will increase as $k$ goes to infinity.
%Then calculate $\Delta e'_k, \Delta z'_k$ for $k \geq n$ to show when .

We start from calculating $\Delta e'_k$ and get $\Delta z'_k$ according to~\eqref{ez}. Since $\lambda, v$ is an eigenvalue and corresponding eigenvector of $A$, we plug in 
$Av=\lambda v$, $K'\Sigma CAv=\lambda K'\Sigma Cv$
in the following proof. For $k=n$ and $k=n+1$, $\Delta e'_k$ satisfies:
\footnotesize
\begin{align*}
\Delta e'_n
=&\tilde{A} \Delta e'_{n-1} - K'y^{a}_{n}                                 
%=\tilde{A}(v+\Delta v) - K'y^{a}_{0}+\lambda K'y^*\\
%=&(A- K'\Sigma CA) \Delta e'_{n-1} - K'y^{a}_{n}\\                                  
%=& (A- K'\Sigma CA) (v+\Delta v) - K'y^{a}_{0}+\lambda K'y^*\\
                                % = &- K'y^{a}_{0}+\lambda v +\tilde{A}\Delta v
                                 %-\lambda K' (\Sigma Cv-y^*)\\
                                 =\Delta e'_{0}+\lambda v +\tilde{A}\Delta v-\lambda K'\Delta y,\\
\Delta e'_{n+1}%=&(\mathbf{A}-\mathbf{K\Sigma CA}) \Delta \mathbf{e}'_{n} - \mathbf{Ky}^{a}_{n+1}\\
                                      % =&(A- K'\Sigma CA) \Delta e'_{n} - K'y^{a}_{1}+\lambda^2 K'y^*\\
                                        % =&\tilde{A} \Delta e'_{n} - K'y^{a}_{1}+\lambda^2 K'y^*\\                                                 
                                      %    =&\Delta e'_{1}+\tilde{A}\lambda v-\lambda^2 K'y^*
                                        %+\tilde{A}^2\Delta v-\lambda\tilde{A} K'\Delta y \\                                                                                 
                                         =&\Delta e'_{1} +\lambda^2 v-\lambda^2 K' \Delta y
                                         +\tilde{A}^2\Delta v-\lambda\tilde{A} K'\Delta y.
\end{align*}
\normalsize
Next we show equation~\eqref{delta_e} holds for $i=0,1,2,\dots$:
\footnotesize
\begin{align}
\begin{split}
\Delta e'_{n+i}
=&\Delta e'_{i} +\lambda^{i+1} v-\lambda^{i+1} K'\Delta y
                                         +\tilde{A}^{i+1}\Delta v-\lambda\tilde{A}^i K' \Delta y,
\end{split}
\label{delta_e}
\end{align}
\normalsize
The above equation~\eqref{delta_e} is true for $i=0$, by induction, assume~\eqref{delta_e} holds for $i$, then for $i+1$, we have:
%\vspace{-10pt}
\footnotesize
\begin{align*}
\Delta e'_{n+i+1}
%&=(A-K'\Sigma CA) \Delta e'_{n+i} - K'y^{a}_{n+i+1}\\
                                  %     &=(A- K'\Sigma CA) \Delta e'_{n+i} - K'y^{a}_{i+1}+\lambda^{i+2} K'y^*\\
                                       &=\tilde{A} \Delta e'_{n+i} - K'y^{a}_{n+i+1}
                                       =\tilde{A}\Delta e'_{n+i} - K'y^{a}_{i+1}+\lambda^{i+2} K'y^*\\
                                        &=\tilde{A} \Delta e'_{i} - K'y^{a}_{i+1}+\lambda^{i+2}K'y^*
                                        +\tilde{A}\lambda^{i+1} v+\tilde{A}\lambda^{i+1} K' \Delta y\\
                                         &\ \ +\tilde{A}^{i+2}\Delta v-\lambda\tilde{A}^{i+1} K' \Delta y \\                                                                                 
                                         &=\Delta e'_{i+1} +\lambda^{i+2}v-\lambda^{i+2} K' \Delta y
                                         +\tilde{A}^{i+2}\Delta v
                                           -\lambda\tilde{A}^{i+1} K' \Delta y.
\end{align*}
\normalsize
Thus we prove that~\eqref{delta_e} holds for $i=0,1,\dots$.

Then plug~\eqref{delta_e} into~\eqref{ez} to calculate $\Delta z'_{n+i}$, we have:
\footnotesize
\begin{align*}
\begin{split}
&\Delta z'_{n+i}
%=&y^a_{i}-\lambda^{i+1}y^*+\Sigma CA(\Delta e'_{i-1} +\lambda^{i} v-\lambda^{i} K' \Delta y\\
                                        % &+\tilde{A}^{i}\Delta v-\lambda\tilde{A}^{i-1} K' \Delta y)\\
                                         =\Delta z'_{i}-\lambda^{i}\Sigma CAK' \Delta y
                                         +\Sigma CA\tilde{A}^{i}\Delta v
                                         -\lambda\Sigma CA\tilde{A}^{i-1} K' \Delta y, 
\end{split}
\end{align*}
\normalsize
and this shows the relation between $\Delta z'_{n+i}$ and $\Delta z'_{i}$. To show how $\Delta z'_{n+i}$ changes when $i$ goes to infinity, we compare $\Delta z'_{n+i}$ with 
$\Delta z'_j$, $0\leq j\leq n-1$ in the following proof.\\  %since $\Delta z'_j$, $0\leq j\leq n-1$ is bounded.
Let $n+i=kn+j, k \geq 1, 0\leq j\leq n-1,$
then: %$\Delta z'_{n+i}$ satisfies:
\footnotesize
\begin{align*}
\begin{split}
\Delta z'_{kn+j}%&\mathbf{y}^a_{i}-\lambda^{i+1}\mathbf{y}^*+\mathbf{CA}(\Delta \mathbf{e}'_{i-1} +\lambda^{i}\mathbf{v}-\lambda^{i}\mathbf{K'}\Delta\mathbf{y}\\
                                        % &+(\mathbf{A}-\mathbf{K'\Sigma CA})^{i}\Delta \mathbf{v}-\lambda(\mathbf{A}-\mathbf{K'\Sigma CA})^{i-1} \mathbf{K'}\Delta\mathbf{y})\\
                                         =&\Delta z'_{(k-1)n+j}-\lambda^{(k-1)n+j}\Sigma CAK' \Delta y\\
                                         &+\Sigma CA\tilde{A}^{(k-1)n+j}\Delta v
                                         -\lambda\Sigma CA\tilde{A}^{(k-1)n+j-1} K' \Delta y\\ 
                                    %    =&\cdots    \\
                                         =&\Delta z'_{j}-\sum\limits_{t=0}^{k-1}[\Sigma CA\tilde{A}^{tn+j}\Delta v
                                         -\lambda\Sigma CA\tilde{A}^{tn+j-1} K' \Delta y]\\
                                         &-\sum\limits_{t=0}^{k-1}\lambda^{tn+j}\Sigma CAK' \Delta y.                                       
\end{split}
\label{deltaz_inf}
\end{align*}
\normalsize
For $0\leq j \leq n-1$, $\|\Delta z'_j\|$ is bounded. 
Under the condition $(A,\Sigma C)$ is detectable, a steady state Kalman filter exists. When we design a steady state kalman filter gain matrix $K'$ for the transformed observer space, such that $\tilde{A}=A-K'\Sigma CA$ is a stable matrix, the last term satisfies:
%$(\Sigma\mathbf{CA}(\mathbf{A}-\mathbf{K'\Sigma CA})^{i}\Delta \mathbf{v}-\lambda\Sigma\mathbf{CA}(\mathbf{A}-\mathbf{K'\Sigma CA})^{i-1} \mathbf{K'}\Delta\mathbf{y})$ 
\begin{center}
$\|\sum\limits_{t=0}^{k-1}[\Sigma CA\tilde{A}^{tn+j}\Delta v
                                         -\lambda\Sigma CA\tilde{A}^{tn+j-1} K'\Delta y]\|_2\leq b$,
                                         \end{center}
where b is some constant scalar. %when $i$ increases.
When $\Sigma CAK' \Delta y \neq 0$, with the unstable eigenvalue $\lambda$ satisfying $\|\lambda\|_2 \geq 1$, we have: 
\begin{center}
$\|\sum\limits_{t=0}^{k-1}\lambda^{tn+j}\Sigma CAK' \Delta y\|_2 \to \infty \ as\  k\to\infty$. 
\end{center}
Under the condition $\Sigma Cv$ is not parallel with $Cv$, when $y*=\epsilon Cv$, $\epsilon \in \mathbb{R}$, we guarantee that $\Delta y =\Sigma Cv-y* \neq 0$.  
\end{proof}
%\end{appendices}
